# Supplementary material for: On mining complex sequential data by means of FCA and pattern structures
Source: arXiv:1504.02255 source file (2015-04-09)
Supplement: Supplementary file 1 [file appendix.tex]

\section*{Appendix}

\begin{proposition}\label{prop:sequential-subsumption}
	Given a sequential pattern structure $(G,(D,\sqcap),\delta)$ and $x,y \in D$, $x$ is subsumed by $y$ ($x \sqsubseteq y$) if and only if for any sequence $s^x \in x$ there is a sequence $s^y \in y$, such that $s^x \leq s^y$
\end{proposition}

\noindent\textbf{Proposition~\ref{prop:proj-and-stability}.} Projections and Stability.
\begin{proof}
	As the concepts extents are equal we refer to these equal sets of objects as ``the extent'' or $Ext$.
	To proof the proposition, one can show that if the closure of any subset of the extent under the projected pattern structure is different from the extent, then the closure of the same set under the original pattern structure is also different from the extent, i.e. for any subset $x \subseteq Ext$, $x^{{\diamond\diamond}_\psi} \neq Ext \rightarrow x^{\diamond\diamond} \neq Ext$. 
	
	If $\tilde{y}=x^{{\diamond\diamond}_\psi}$ is not equal to $Ext$ then there is a concept $\tilde{c_y}$ for $(G,(D_\psi,\sqcap_\psi),\psi \circ \delta)$ with the extent equal to $\tilde{y}$. According to Proposition~\ref{prop:proj-and-concepts} there is a concept $c_y$ for $(G,(D,\sqcap),\delta)$ with the same extent $\tilde{y}$. As $x \subseteq y$ then $x^{\diamond\diamond} \subseteq y \subset Ext$, i.e. $x^{\diamond\diamond} \neq Ext$
\end{proof}

\noindent\textbf{Proposition~\ref{prop:proj-MLP}.} MLP is a monotone, contractive and idempotent.
\begin{proof}
	The contractivity and idempotentcy are quite clear from the definition. Remains the proof for monotonicity.
	
	If $X \sqsubseteq Y$ where $X$ and $Y$ are sets of sequences then for every sequence $x \in X$ there is a sequence $y \in Y$ such that $x \leq y$ (Proposition~\ref{prop:sequential-subsumption}). We should show that $\psi_l(X) \sqsubseteq \psi_l(Y)$, or in other words for every sequence $x\in \psi_l(X)$ there is a sequence $y$ in $\psi_l(Y)$, such that $x\leq y$. Given $x \in \psi_l(X)$, as $\psi_l(X)$ is a subset of $X$ and as $X \sqsubseteq Y$, the there is a sequence $y\in Y$ such that $x \leq y$, with $|y| \geq |x| \geq l$, and thus, $y \in \psi_l(Y)$.
\end{proof}

\noindent\textbf{Proposition~\ref{prop:proj-alphabet-proj}.} Alphabet lattice projection is a projection of the pattern structure.
\begin{proof}
	$\psi_{\psi_E}$ is idempotent, since the projection of the alphabet is idempotent. $\psi_{\psi_E}$ is contractive because the projection of a sequence $\tilde{s}$ is a subsequence of the sequence $s$ (``restricted'' Definition~\ref{def:subsequence}), i.e. $\{\tilde{s}\}$ is subsumed by $\{s\}$. In the Definition~\ref{def:pattern-alph-proj} the sequences should be cut on the top elements of the alphabet lattice, building the sets $\{\tilde{s}^i\}$ and $\{s^j\}$. In these sets there is no `TOP' element of the alphabet, thus, for any $\tilde{s}^i$ there is a supersequence $s^j$, and, so, the projected pattern $\tilde{d}=\psi_{\psi_E}(d)$ is subsumed by the pattern $d$ ($\tilde{d}\sqsubseteq d$). The last thing for showing is that the alphabet projection is monotone.
	
	For two patterns $x,y \in D$, such that $x \sqsubseteq y$, i.e. $\forall s^x \in x \exists s^y \in y: s^x \leq s^y$, consider the projected sequence of $s^x$, $\psi_{\psi_E}(s^x)$. As $s^x \leq s^y$ for some $s^y$ then for some $k \in \set{0\+1\+...\+|s^y| - |s^x|}$ and $j_i = k+i$ (see Definition~\ref{def:subsequence}) $s^x_i \sqsubseteqe s^y_{j_i}$ ($i \in {1,2,...,|s^x|}$), then $\psi_E(s^x_i) \sqsubseteqe \psi_E(s^y_{j_i})$ (by the property of the alphabet projection), i.e. projected sequence preserve the subsequence relation. Thus, the alphabet projection of the pattern preserve pattern subsumption relation, $\psi_{\psi_E}(\{x\}) \leq \psi_{\psi_E}(\{y\})$ (Proposition~\ref{prop:sequential-subsumption}), i.e. the alphabet projection is monotone.
\end{proof}
